# Supplementary material for: Multiple Contexts and Frequencies Aggregation Network forDeepfake Detection
Source: arXiv:2408.01668 source file (2024-08-03)
Supplement: Supplementary file 1 [file supp_other_choice_forgery_TS.tex]

\begin{table*}
  \centering
  \scalebox{0.65}{
  \begin{tabular}{c|c|c|c|c|c|c} \toprule
    \multirow{2}*{Encoder Architecture} & DFD & CDF-v1 & CDF-v2 & DFDCP & DFDC & Avg.\\ 
    \cmidrule(lr){2-2}
    \cmidrule(lr){3-3}
    \cmidrule(lr){4-4}
    \cmidrule(lr){5-5}
    \cmidrule(lr){6-6}
    \cmidrule(lr){7-7}
    & AUC~$\uparrow$ ~\textbar~ AP~$\uparrow$ ~\textbar~ EER~$\downarrow$ & AUC~$\uparrow$ ~\textbar~ AP~$\uparrow$ ~\textbar~ EER~$\downarrow$ & AUC~$\uparrow$ ~\textbar~ AP~$\uparrow$ ~\textbar~ EER~$\downarrow$ & AUC~$\uparrow$ ~\textbar~ AP~$\uparrow$ ~\textbar~ EER~$\downarrow$ & AUC~$\uparrow$ ~\textbar~ AP~$\uparrow$ ~\textbar~ EER~$\downarrow$ & AUC~$\uparrow$ ~\textbar~ AP~$\uparrow$ ~\textbar~ EER~$\downarrow$ \\
    \midrule
    Xception & \textbf{0.888} ~\textbar~ \textbf{0.986} ~\textbar~ 20.3 & 0.823 ~\textbar~ 0.884 ~\textbar~ 23.5 & 0.806 ~\textbar~ 0.882   ~\textbar~ 27.1 & 0.796   ~\textbar~ 0.887 ~\textbar~ 28.5 & 0.729 ~\textbar~ 0.752 ~\textbar~ 34.0 & 0.808 ~\textbar~ 0.878 ~\textbar~ 26.7 \\
    
    EfficientNet-B1 & 0.870 ~\textbar~ 0.983 ~\textbar~ 21.4 & 0.821 ~\textbar~ 0.885 ~\textbar~ 25.1 & 0.809 ~\textbar~ 0.882 ~\textbar~ 27.2 & 0.789 ~\textbar~ 0.881 ~\textbar~ 28.6 & 0.733 ~\textbar~ 0.756 ~\textbar~ 33.5 & 0.804 ~\textbar~ 0.877 ~\textbar~ 27.2 \\

    EfficientNet-B4 & 0.880 ~\textbar~ 0.984 ~\textbar~ \textbf{20.0} & \textbf{0.867} ~\textbar~ \textbf{0.922} ~\textbar~ \textbf{21.9} & 0.830 ~\textbar~ \textbf{0.904} ~\textbar~ \textbf{25.9} & \textbf{0.815} ~\textbar~ \textbf{0.893} ~\textbar~ \textbf{26.9} & 0.736 ~\textbar~ 0.760 ~\textbar~ \textbf{33.0} & \textbf{0.825} ~\textbar~ \textbf{0.893} ~\textbar~ \textbf{25.5} \\
    
    EfficientNet-B5 & 0.877 ~\textbar~ 0.984 ~\textbar~ 21.0 & 0.848 ~\textbar~ 0.919 ~\textbar~ 22.0 & \textbf{0.833} ~\textbar~ 0.898 ~\textbar~ 25.7 & 0.812 ~\textbar~ 0.892 ~\textbar~ 27.1 & \textbf{0.748} ~\textbar~ \textbf{0.772} ~\textbar~ 32.4 & 0.824 ~\textbar~ \textbf{0.893} ~\textbar~ 25.6 \\
    
    \bottomrule
  \end{tabular}
  }
  \caption{
  Performance evaluation of different encoder architectures. All models are trained on the FF++\_c23 dataset and evaluated across various other datasets with metrics presented in the order of AUC~\textbar~AP~\textbar~EER (the frame-level). The average performance (Avg.) across all datasets is also reported. The best results are highlighted in bold.
  }
  \label{tab:other-choice-backbone}
\end{table*}
