# Supplementary material for: Multiple Contexts and Frequencies Aggregation Network forDeepfake Detection
Source: arXiv:2408.01668 source file (2024-08-03)
Supplement: Supplementary file 2 [file supp_within_entire_synthesis.tex]

\begin{table}[tb!]
  \centering
%   \vspace{1mm}
  \scalebox{0.75}{
  \begin{tabular}{c|c|c|c|c}
    \toprule
    \multirow{2}*{Method}
    &\multicolumn{4}{c}{Testing Datasets}\\
    \cmidrule(lr){2-5}
    & StarGAN~\cite{choi2018stargan} & DDPM~\cite{ho2020denoising} & DDIM~\cite{song2020denoising} & SD~\cite{rombach2022high} \\
    \midrule
    
    SBI~\cite{shiohara2022detecting} & 0.787 & 0.744 & 0.648 & 0.478 \\

    \midrule

    Ours & \textbf{0.810} &  \textbf{0.854}& \textbf{0.748} & \textbf{0.506} \\
     \bottomrule
  \end{tabular}}
  \caption{
  Results in detecting GAN-generated images and Diffusion-generated images. We compare our results with other augmentation-based SBI~\cite{shiohara2022detecting}. We utilize its official code for evaluation. These models are trained on FF++\_c23. The metric used is the frame-level AUC. ``SD" is the short for stable diffusion.
  }
  \vspace{-10pt}
  \label{tab:ablation_within_entire_synthesis}
\end{table}
